# Supplementary material for: MemControl: Mitigating Memorization in Diffusion Models via Automated Parameter Selection
Source: arXiv:2405.19458 source file (2025-02-11)
Supplement: Supplementary file 1 [file appendix.tex]

% \title{Supplementary Material}
\author{}
\date{}

% \begin{document}

\maketitle

\section{Analysis of the Compute Cost} \label{sec:compute_cost}

In this section, we analyze the compute cost of our approach and the different baselines. We use hyperparameter optimization (HPO) for each of them. Each HPO trial was conducted on 1\% of the original MIMIC dataset (1100 samples) combined with 100 image-text pairs from the memorization subset, repeated 50 times (5000 samples), resulting in a total of 6100 samples. Each trial consisted of 3000 optimization steps with a batch size of 128, requiring 2 GPU hours (GPUh) per iteration on an NVIDIA V100 GPU. In total, we ran 30 trials for \textit{MemControl}, amounting to 60 GPU hours for the entire process. 
% For a fair comparison, we compared our results with tuned baselines (Full FT) that required 10 similar HPO trials to determine the optimal learning rate, totalling 20 GPU hours. Table \ref{tab:compute_cost} summarizes the compute requirement for each experiment and baseline.
We compare our approach with tuned baselines. For example, full FT required 10 similar HPO trials to determine the optimal learning rate, totalling 20 GPU hours. Table \ref{tab:compute_cost} summarizes the compute requirement for each experiment and baseline.

\begin{table}[h]
\centering
\resizebox{0.45\textwidth}{!}{%
\begin{tabular}{lc}
\toprule
% \rowcolor[HTML]{CBCEFB}
\textbf{Method}                                                                                                        & \textbf{\begin{tabular}[c]{@{}c@{}}Compute Cost\end{tabular}}  \\ \midrule
\begin{tabular}[c]{@{}c@{}}Full FT/ SV-DIFF/ DiffFit/ Attention (Tuned Baseline)\end{tabular}                        & 20 hours                                                                    \\ 
\begin{tabular}[c]{@{}c@{}}Full FT/ SV-DIFF/ DiffFit/ Attention + RWA(Tuned Baseline)\end{tabular}                  & 27 hours                                                                    \\
\begin{tabular}[c]{@{}c@{}}Full FT/ SV-DIFF/ DiffFit/ Attention + Threshold Mitigation (Tuned Baseline)\end{tabular} & 35 hours                                                                    \\
\textit{MemControl (ours)}                                                                   & 60 hours     \\ \bottomrule           
\end{tabular}
}
\caption{An analysis of the compute cost in GPU hours for the different fine-tuning and memorization mitigation strategies. \textit{Tuned Baseline} refers to the baseline obtained after searching for the optimal learning rate and other hyperparameters.}
\label{tab:compute_cost}
\end{table}

\section{Further Discussion on Experimental Details and Results}

\subsection{Creating the Memorization Subset} \label{sec:mem_subset}

\begin{figure*}[ht]
  \centering
    \includegraphics[width=0.9\linewidth]{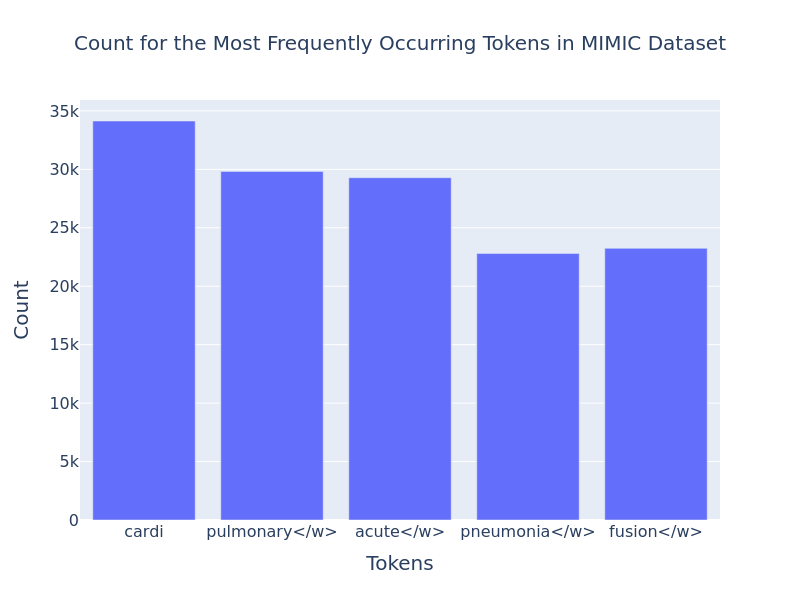}
  \caption{Count for the most frequently occurring tokens in the MIMIC dataset.
  }
  \label{fig:memorized_token_count_bar_plot}
\end{figure*}

The memorization subset was created with the objective of forcing the model to memorize specific image-text pairs within the dataset during training and measuring memorization on these specific samples for reporting to the HPO. First, we identified the most frequently occurring tokens within all text captions in the MIMIC dataset (Figure \ref{fig:memorized_token_count_bar_plot}). As a next step, we selected 100 text captions having the highest count of these particular tokens. These 100 image-text pairs constituted our \textit{memorization subset}. During training, this subset was duplicated 50 times resulting in 5000 additional samples.

\subsection{Results with Random Word Addition (RWA)} \label{sec:RWA}
Random Word Addition (RWA) has been proposed as a successful mitigation strategy in \cite{somepalli2023understanding}. The method involves replacing tokens/words in the caption with a random word. This method turned out to be the most successful mitigation strategy in the analysis performed in \cite{somepalli2023understanding}. However, our results indicate that RWA often leads to a substantial decrease in generative performance. A simple explanation for this observation is that medical vocabulary, and hence prompts in a medical dataset, are very different from those in a dataset containing natural images. Since the stable diffusion pipeline uses a tokenizer trained on \textit{natural} prompts, it often lacks significant knowledge about the specific medical terminology used in medical datasets. RWA works by generating a random integer (between 0 and 49,400) and decoding that integer into the corresponding text token using the tokenizer. 
With a non-medical tokenizer, the random word that is added often decreases the quality of the caption which in turn significantly impacts the textual guidance in generating new images. 
Although RWA did decrease memorization in certain cases in our experiments, it came at the cost of lower generation quality.

\newpage
\section{Elucidating the Parameter Search Space} \label{sec:search_space}

Our framework performs a hyperparameter search to identify the optimal locations for fine-tuning or model components for adding specific PEFT parameters. This process utilizes a binary mask where each element's position corresponds to a specific component in the Stable Diffusion U-Net. The element's value (0 or 1) indicates whether the parameter at that location should be frozen or fine-tuned. A similar investigation was conducted in \cite{xiang2023closer}, which found that modulating the placement of PEFT parameters around cross-attention blocks in the U-Net yields the best performance. Building on this insight, we constrain our search space to include both self-attention and cross-attention blocks in the U-Net for each PEFT method.

\textbf{Stable Diffusion U-Net Design: } The Stable diffusion U-Net is a modified version of the original model \cite{ronneberger2015u} with additional self-attention and cross-attention blocks for textual guidance. Architecturally, the model is divided into 4 \textit{down-blocks}, 1 \textit{mid-block}, and 4 \textit{up-blocks}. The self-attention and cross-attention blocks are contained in the \textit{mid-block}, more specifically in the first and the last three down and up blocks respectively.

\subsection{Search Space for SV-DIFF}

SV-DIFF \cite{han2023svdiff} starts by conducting a Singular Value Decomposition (SVD) on the weight matrices of a pre-trained diffusion model as a one-time calculation. During fine-tuning, the original weight matrices are kept frozen, and only the \textit{spectral shift} parameters are updated, resulting in a very small number of parameters being adjusted (0.02\% of the total parameters in the U-Net). In its original setup, SV-DIFF is applied to the weight matrices of all U-Net layers (including Conv1D, Conv2D, Linear, Embedding, LayerNorm, and GroupNorm). Building on the brief investigation in \cite{han2023svdiff} regarding the fine-tuning of spectral shifts within specific parameter subsets of the U-Net, we define our search space to include all self-attention and cross-attention blocks within the U-Net.

Given that there are 6 attention blocks (3 self-attention and 3 cross-attention) in both  \textit{down-blocks} and \textit{up-blocks}, and 1 attention block in the \textit{mid-block}, our search space for the binary mask is \(\Omega \in \{0,1\}^{13}\). For a binary mask of length 13, the first 6 elements represent the \textit{down-blocks}, the next 6 elements denote the \textit{up-blocks}, and the other element corresponds to the \textit{mid-block}.

\subsection{Search Space for DiffFit}
DiffFit PEFT strategy \cite{xie2023difffit} introduces learnable scale parameters $\gamma$ into the diffusion model blocks. During fine-tuning, the majority of the model is frozen and only the bias, normalization, class-condition module and the learnable parameters $\gamma$ are updated.

Similar to SV-DIFF, we explore the various positions for adding DiffFit parameters in the attention blocks of the U-Net. Given that there are 6 attention blocks (3 self-attention and 3 cross-attention) in both \textit{down-blocks} and \textit{up-blocks}, and 1 attention block in the \textit{mid-block}, our search space for the binary mask is \(\Omega \in \{0,1\}^{13}\). For a binary mask of length 13, the first 6 elements represent the \textit{down-blocks}, the next 6 elements denote the \textit{up-blocks}, and the other element corresponds to the \textit{mid-block}.

\section{Experimental Settings for Hyperparameter Optimization (HPO)} \label{sec:hpo_analysis}

\textbf{Parameter Sampler:} We use the NSGA-II algorithm \cite{NGSAII_sampler} to sample hyperparameter values. Initially, an initial population of random solutions is generated. The objective functions are then evaluated on each solution in the population. Finally, the candidate solutions are sorted according to Pareto dominance. The algorithm maintains diversity by giving preference to solutions in less crowded regions.

% TPE fits a Gaussian Mixture Model (GMM) to the parameter values (binary mask, in our case) that yield the best results for the objective metric (e.g., memorization metric $d^{mem}$ and FID Score). Consequently, with each trial, we sample better parameters (masks) that lead to improved objective values.

\textbf{Bi-level  Optimization Using NSGA-II:} In each trial, the NSGA-II sampler selects values for the binary mask to be used for fine-tuning. After fine-tuning, we obtain a value for the objective metric associated with the sampled mask values. Over numerous trials, the sampler identifies which values better optimize the objective metric and gives these values higher preference in the sampling process. In the case of single-objective optimization, pruning techniques such as Successive Halving (SH) can be employed for early termination of unpromising trials.

\textbf{Scalability to Large Datasets: }  Employing our framework on the MIMIC dataset consisting of 110K training samples enabled us to test the scalability of our framework to large datasets. We randomly sampled 1\% (1,100 samples) from the dataset for the HPO search, and the mask obtained on this subset was finally used for fine-tuning on the entire dataset. Previously, such sampling strategies for conducting HPO search on large datasets have been shown to be effective \cite{dutt2024fairtune, shim2021core, visalpara2021data}.

\subsection{Analysis of the HPO}

In this section, we present an analysis of the HPO search over different PEFT search spaces. 

\textbf{Convergence of the HPO: } Figure \ref{fig:optimization_history} illustrates the outer loop convergence in the bi-level optimization for the specific case of the SV-DIFF parameter search space. The plot demonstrates that the memorization metric \(d^{mem}\) successfully converges for both parameter search spaces (SV-DIFF and DiffFit) within the given number of outer loop iterations. This indicates that the HPO search ran for a sufficient number of trials to reach the optimal objective value.

% \begin{figure}[h]
%   \centering
%     \includegraphics[width=1.5\linewidth, height=2.5in]{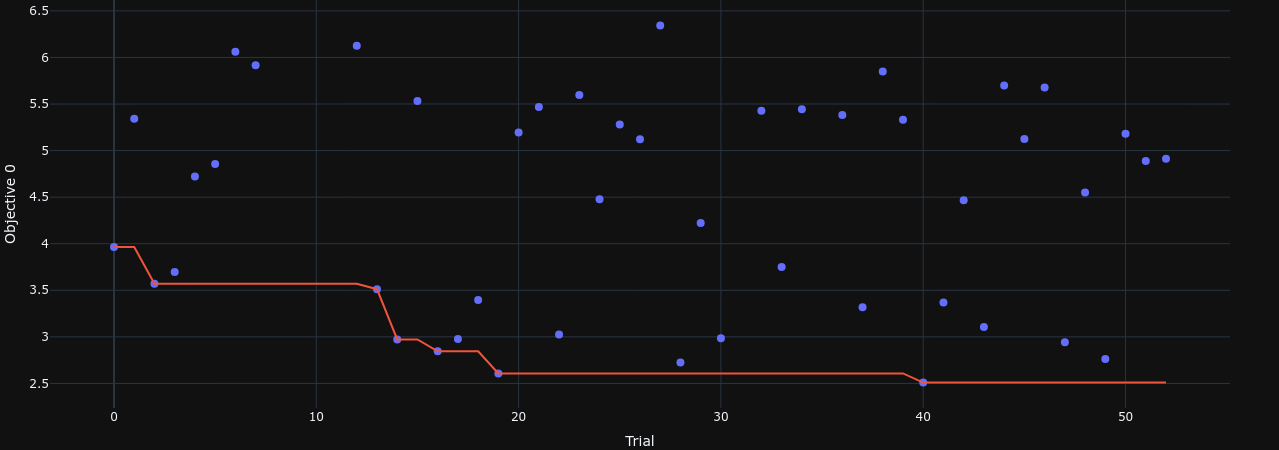}
%   \caption{Figure depicting the optimization history of the memorization metric during the HPO search for SV-DIFF method.
%   }
%   \label{fig:optimization_history}
% \end{figure}

\begin{figure*}[htbp] 
    \centering
    \includegraphics[width=\textwidth]{assests/Optimization_History_Memorization_Metric.png} 
    \caption{Figure depicting the optimization history of the memorization metric during the HPO search for SV-DIFF method. It can be observed that the HPO converged (no improvement in the objective metric) around the 18th trial.}
    \label{fig:optimization_history}
\end{figure*}

%%%%%%%%% REFERENCES
% {\small
% \bibliographystyle{ieee_fullname}
% \bibliography{references}
% }
% \printbibliography

% \end{document}
